# Supplementary material for: Multi-intent-aware Session-based Recommendation
Source: arXiv:2405.00986 source file (2024-05-02)
Supplement: Supplementary file 1 [file sec-appendix.tex]

% Technical Appendix (https://aaai.org/aaai-conference/aaai-24-supplementary-material/)
% The length of main submissions is strictly limited, as already described. Authors may optionally submit a technical appendix (PDF) containing additional supporting information such as proofs of theorems that are stated in the main paper; additional information needed to reproduce experiments; further experimental results; figures and examples to illustrate technical claims; etc. The main submission may reference the supplementary material, but should be self contained. Reviewers will be instructed to make their acceptance evaluations based on the main submission, and will not be obliged to consult the supplementary material. If proofs or other supplementary matter are an important part of the contribution, their essential elements should be included in the main paper.

\appendix

\section{Reproducibility}

\begin{table}[]
\centering
\begin{tabular}{c|ccccc}
\toprule
Dataset & $\tau$ & $\delta_{tr}$ & $\delta_{emb}$ & $\alpha$ & $\beta$ \\ \midrule
Dginetica & 0.07 & 0.1 & 0.1 & 1.5 & 0.9 \\
Retailrocket & 0.07 & 0.1 & 0.1 & 1.5 & 0.8 \\
Yoochoose & 0.07 & 0.1 & 0.1 & 1.5 & 0.7 \\
Tmall & 0.05 & 0.1 & 0.1 & 1.5 & 0.5 \\
Dressipi & 0.07 & 0.1 & 0.1 & 1.5 & 0.9 \\
LastFM & 0.07 & 0.1 & 0.1 & 1.5 & 0.8 \\
\bottomrule
\end{tabular}
\caption{Optimal hyperparameters of EDISON for each dataset.}\label{tab:optimal_hyper}
\end{table}
Table~\ref{tab:optimal_hyper} shows EDISON's optimal hyperparameters for each dataset. In addition, hyperparameters that were fixed and experimented with, such as the batch size and the dimension of the embedding vectors, can be found in the Experimental Setup section of the main paper. 

\section{Additional Experimental Results}

\subsection{Performance Comparison}\label{sec:exp_hyper}
\begin{table*} \small
\centering
\setlength{\tabcolsep}{2.5pt}

\begin{tabular}{c|c|cccccc|cccc|c|r}
\toprule
Dataset & Metric & SASRec & SR-GNN & NISER+ & SGNN-HN & DSAN & CORE & SINE & A-mixer & ComiRec & Re4 & EDISON & \multicolumn{1}{c}{Imp.} \\ \midrule
\multirow{2}{*}{Diginetica} & R@5 & 25.73 & 25.01 & 27.48 & 26.46 & 27.88 & \ul{ 28.51} & 24.07 & 25.01 & 27.62 & 27.91 & \textbf{29.30$^{\ddagger}$} & 2.77\% \\
 & M@5 & 14.84 & 14.33 & 15.87 & 14.89 & 15.85 & 16.12 & 13.91 & 14.30 & 16.02 & \ul{ 16.14} & \textbf{16.92$^{\dagger}$} & 4.88\% \\ \midrule
\multirow{2}{*}{Retailrocket} & R@5 & 45.03 & 45.88 & 48.13 & 45.11 & \ul{ 48.45} & 48.12 & 42.50 & 45.42 & 48.35 & 48.39 & \textbf{49.94$^{\ddagger}$} & 3.08\% \\
 & M@5 & 34.21 & 34.75 & 36.89 & 34.12 & \ul{ 37.37} & 37.09 & 32.87 & 34.87 & 36.80 & 36.74 & \textbf{38.00$^{\ddagger}$} & 1.69\% \\ \midrule
\multirow{2}{*}{Yoochoose} & R@5 & 43.41 & 42.86 & 43.46 & 41.65 & 43.75 & \ul{ 44.10} & 37.69 & 42.37 & 42.44 & 43.05 & \textbf{44.31} & 0.48\% \\
 & M@5 & 26.51 & 26.31 & 26.94 & 25.86 & \ul{ 27.11} & 26.08 & 23.00 & 25.86 & 25.91 & 26.17 & \textbf{27.52} & 1.51\% \\ \midrule
\multirow{2}{*}{Tmall} & R@5 & 29.21 & 28.56 & 34.59 & 30.82 & 36.70 & \ul{ 37.86} & 27.64 & 33.79 & 34.05 & 34.54 & \textbf{43.25$^{\ddagger}$} & 14.25\% \\
 & M@5 & 24.41 & 24.25 & 28.88 & 23.25 & 30.22 & \ul{ 30.85} & 26.69 & 27.76 & 27.18 & 27.62 & \textbf{32.37$^{\ddagger}$} & 4.90\% \\ \midrule
\multirow{2}{*}{Dressipi} & R@5 & 21.21 & 21.55 & 22.91 & 22.84 & 22.46 & 23.24 & 23.11 & 20.72 & \ul{ 24.38} & 24.12 & \textbf{25.10$^{\dagger}$} & 2.95\% \\
 & M@5 & 12.72 & 13.05 & 13.81 & 13.49 & 13.60 & 14.04 & 13.95 & 12.34 & \ul{ 14.53} & 14.40 & \textbf{14.67$^{\dagger}$} & 0.99\% \\ \midrule
\multirow{2}{*}{LastFM} & R@5 & 9.56 & 11.78 & 12.01 & 11.38 & 11.45 & 11.64 & 11.19 & 10.62 & 11.52 & \ul{ 12.38} & \textbf{13.73$^{\ddagger}$} & 10.85\% \\
 & M@5 & 5.17 & 7.74 & \ul{ 7.79} & 6.57 & 6.87 & 6.77 & 6.52 & 6.49 & 6.81 & 7.47 & \textbf{8.18$^{\dagger}$} & 5.05\% \\
\bottomrule
\end{tabular}
\caption{Performance comparison for the proposed method and baseline models. Imp. indicates how much better EDISON is than the best baseline model. The best model is marked bold and the second best model is underlined. Significant differences ($\rho < 0.05$ and $\rho < 0.01$) between the best baseline model and EDISON are reported with $\dagger$ and $\ddagger$.}\label{tab:exp_all_cutoff5}
\end{table*}

Table~\ref{tab:exp_all_cutoff5} shows the accuracy of the baseline models and EDISON when the cutoff is 5. EDISON consistently outperforms all baseline models at various cutoffs of 20, 10, and 5. Additionally, most other observations are similar regardless of the cutoff, \eg, EDISON's gain in accuracy over the comparison models is highest for Tmall and LastFM, and the accuracy of CORE is among the highest of the baselines. 

\subsection{Effect of Hyperparameters}\label{sec:exp_hyper}
\begin{figure*}[t]
\centering
\begin{tabular}{ccc}
\includegraphics[width=0.3\textwidth]{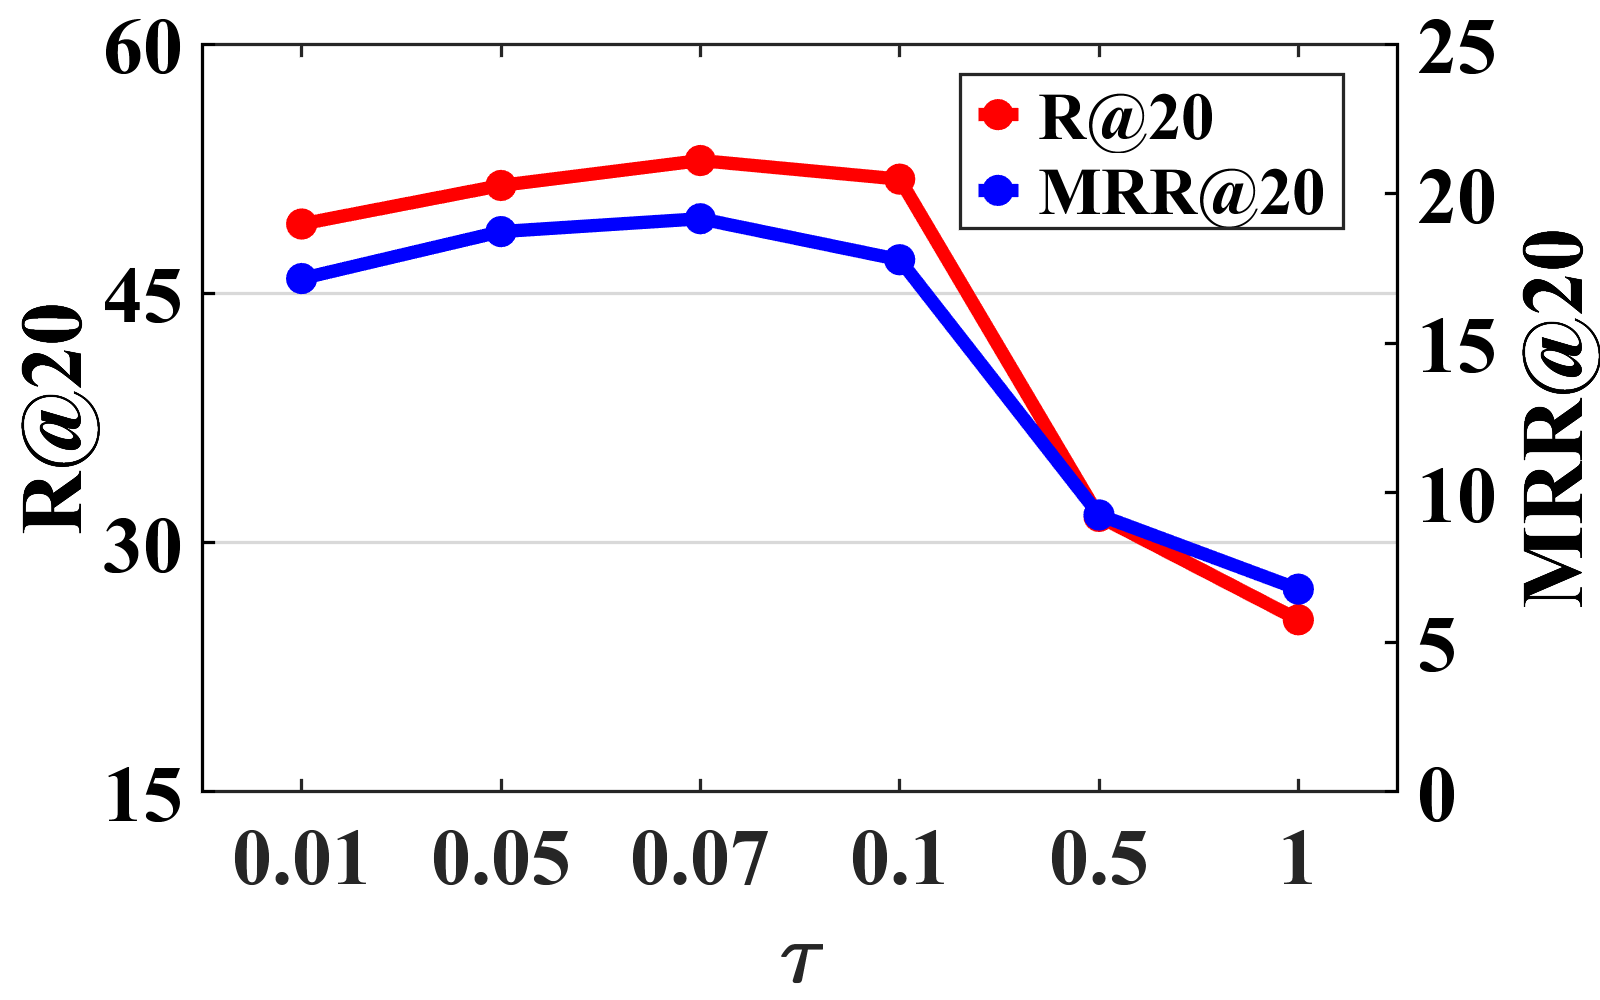} &
\includegraphics[width=0.3\textwidth]{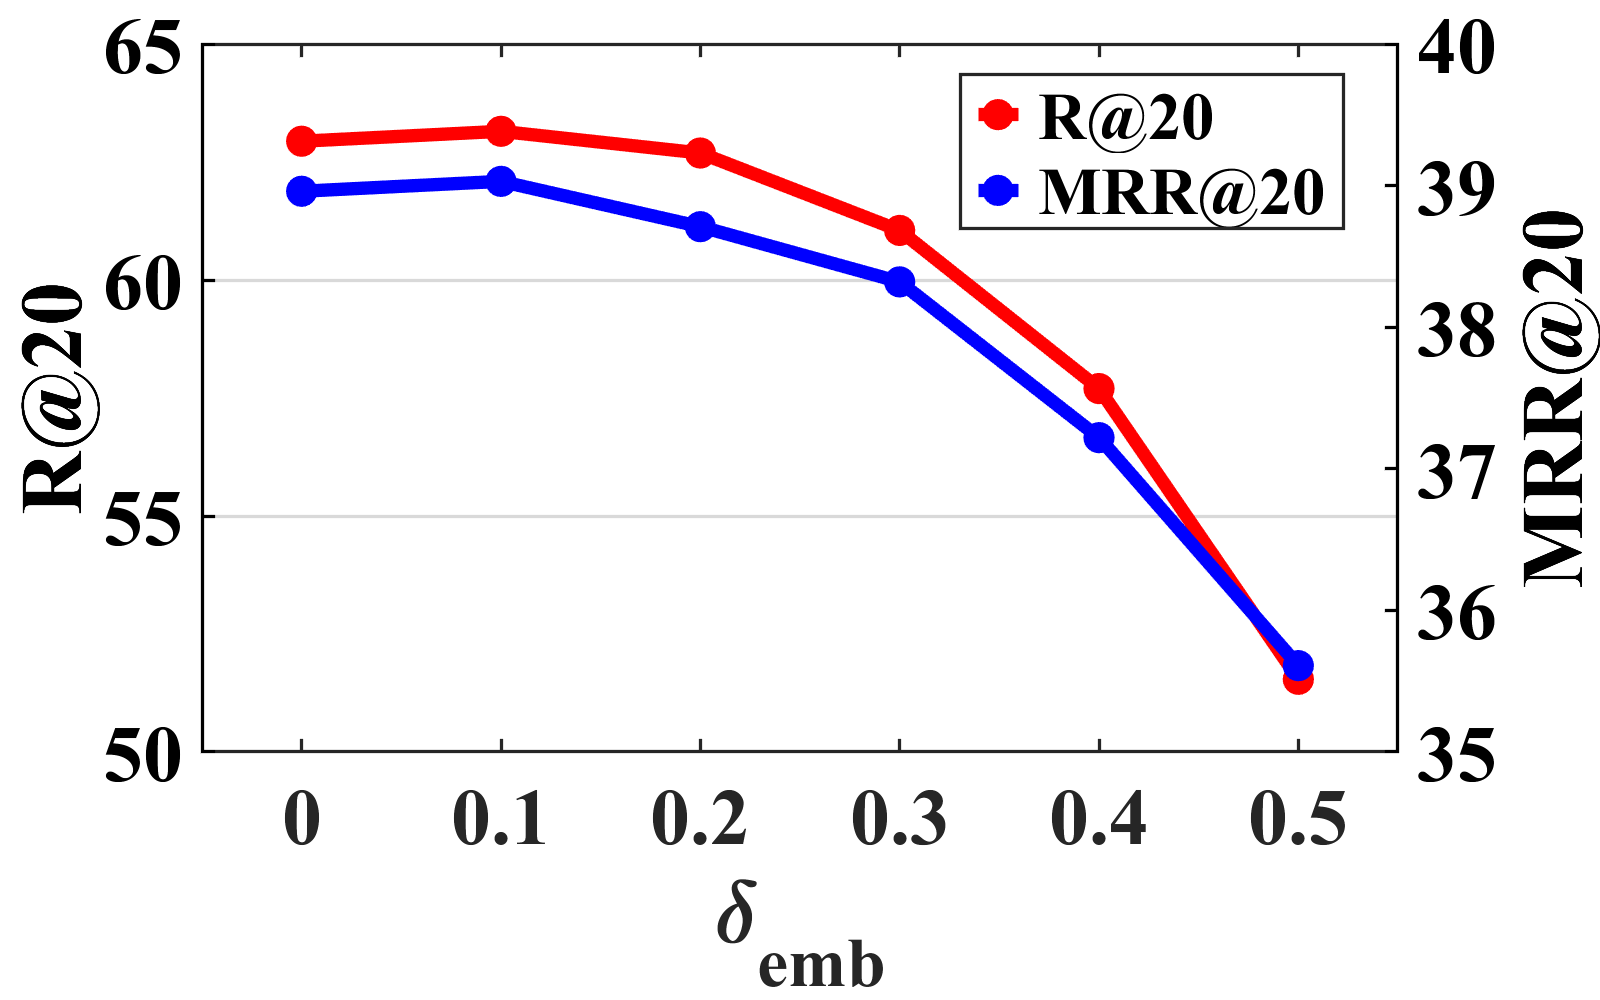} &
\includegraphics[width=0.3\textwidth]{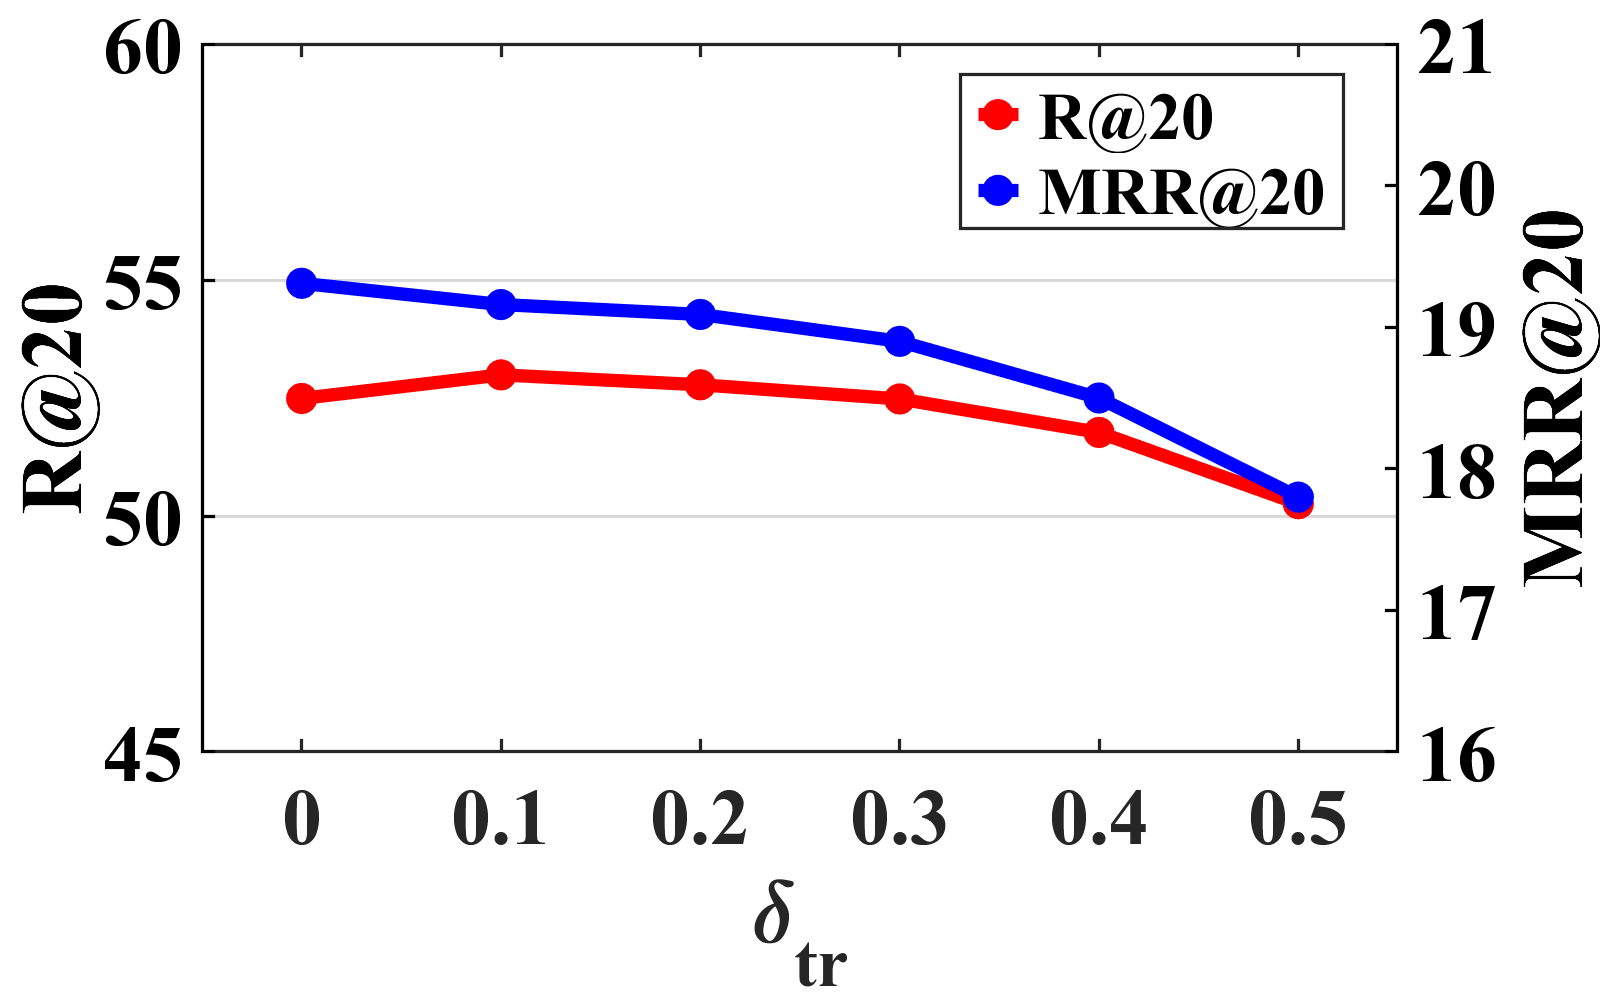} \\
\end{tabular} \\
(a) Diginetica \\

\begin{tabular}{ccc}
\includegraphics[width=0.3\textwidth]{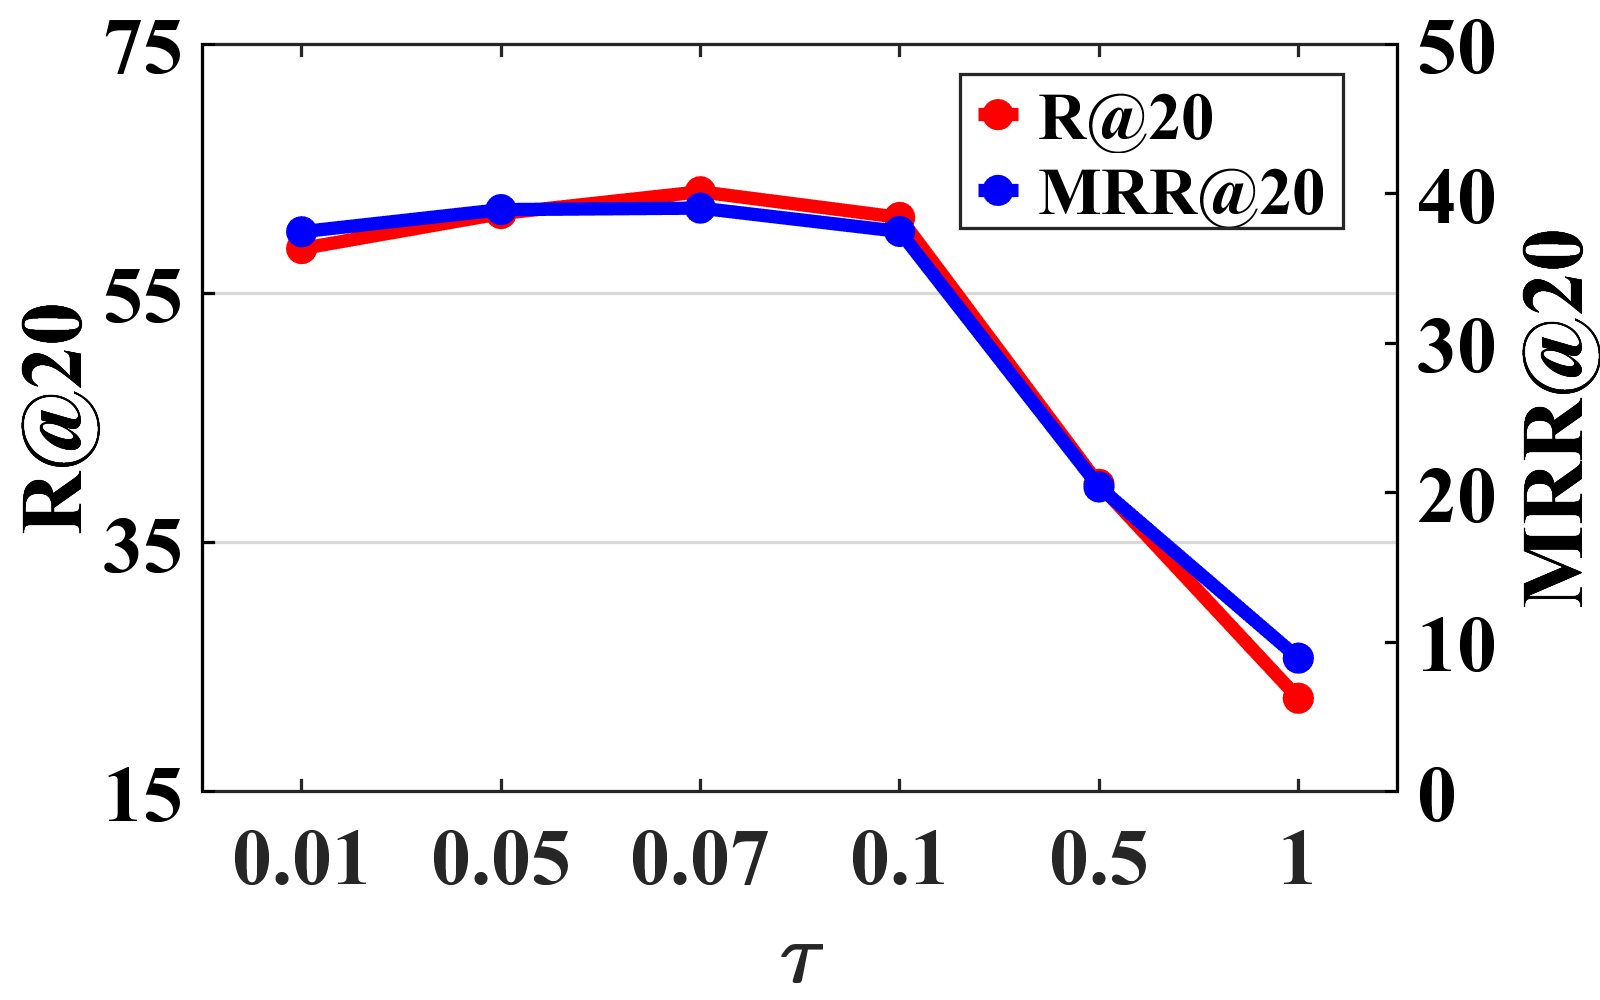} &
\includegraphics[width=0.3\textwidth]{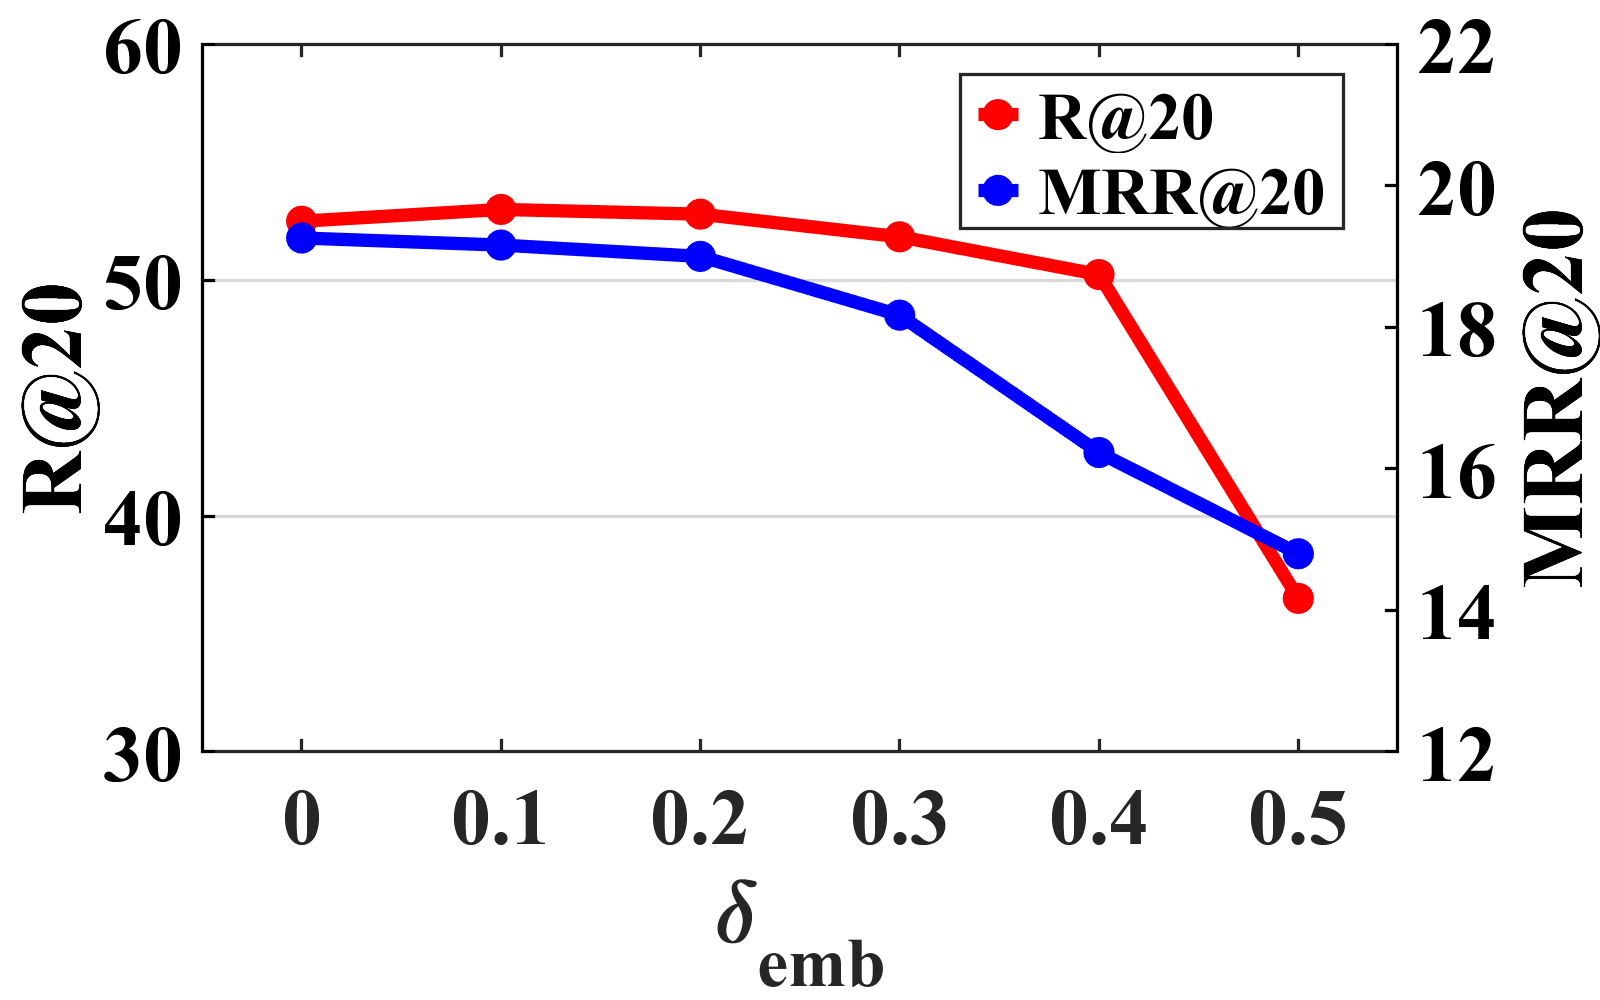} &
\includegraphics[width=0.3\textwidth]{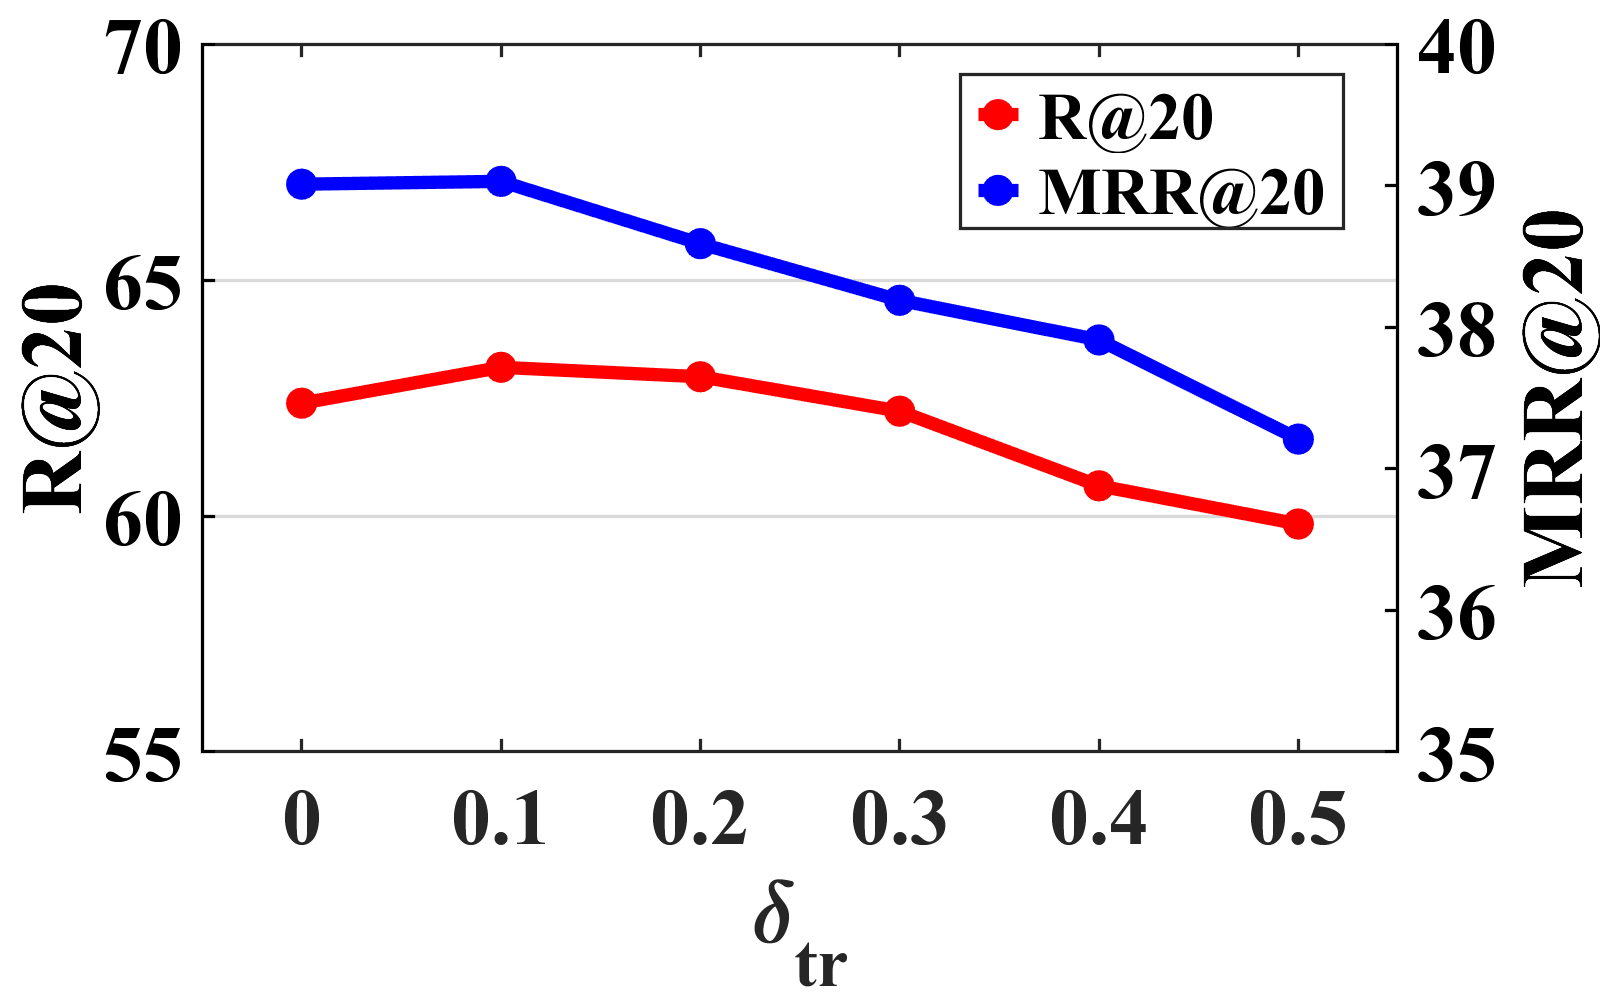} \\
\end{tabular} \\
(b) Retailrocket  \\

\begin{tabular}{ccc}
\includegraphics[width=0.3\textwidth]{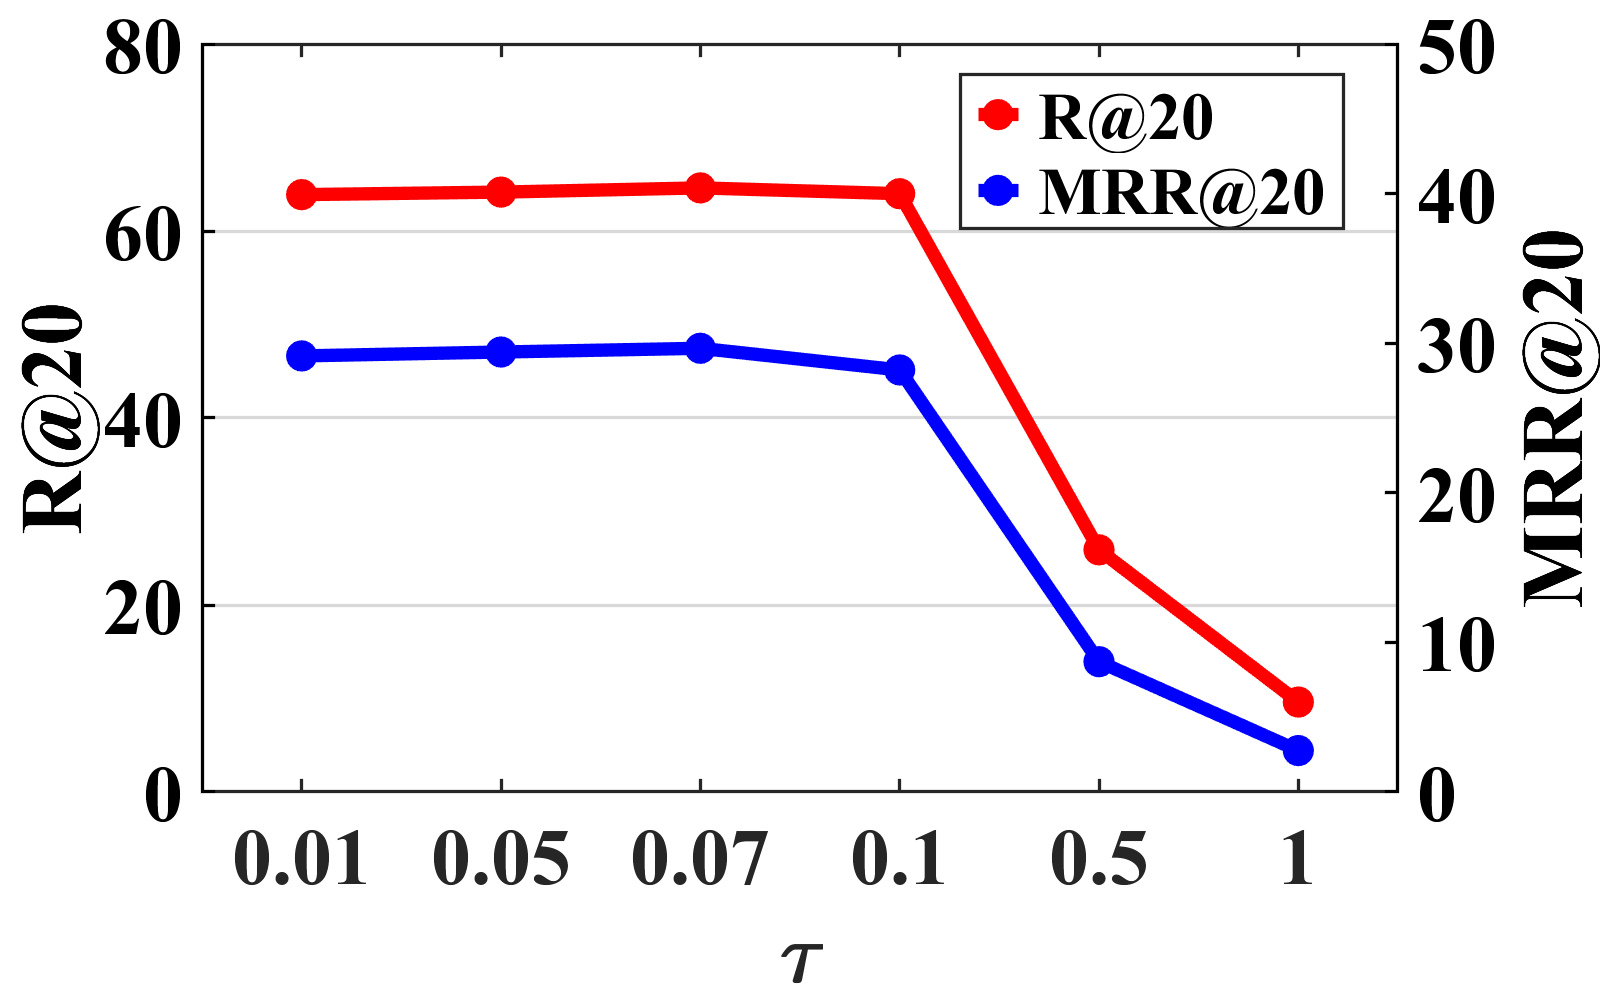} &
\includegraphics[width=0.3\textwidth]{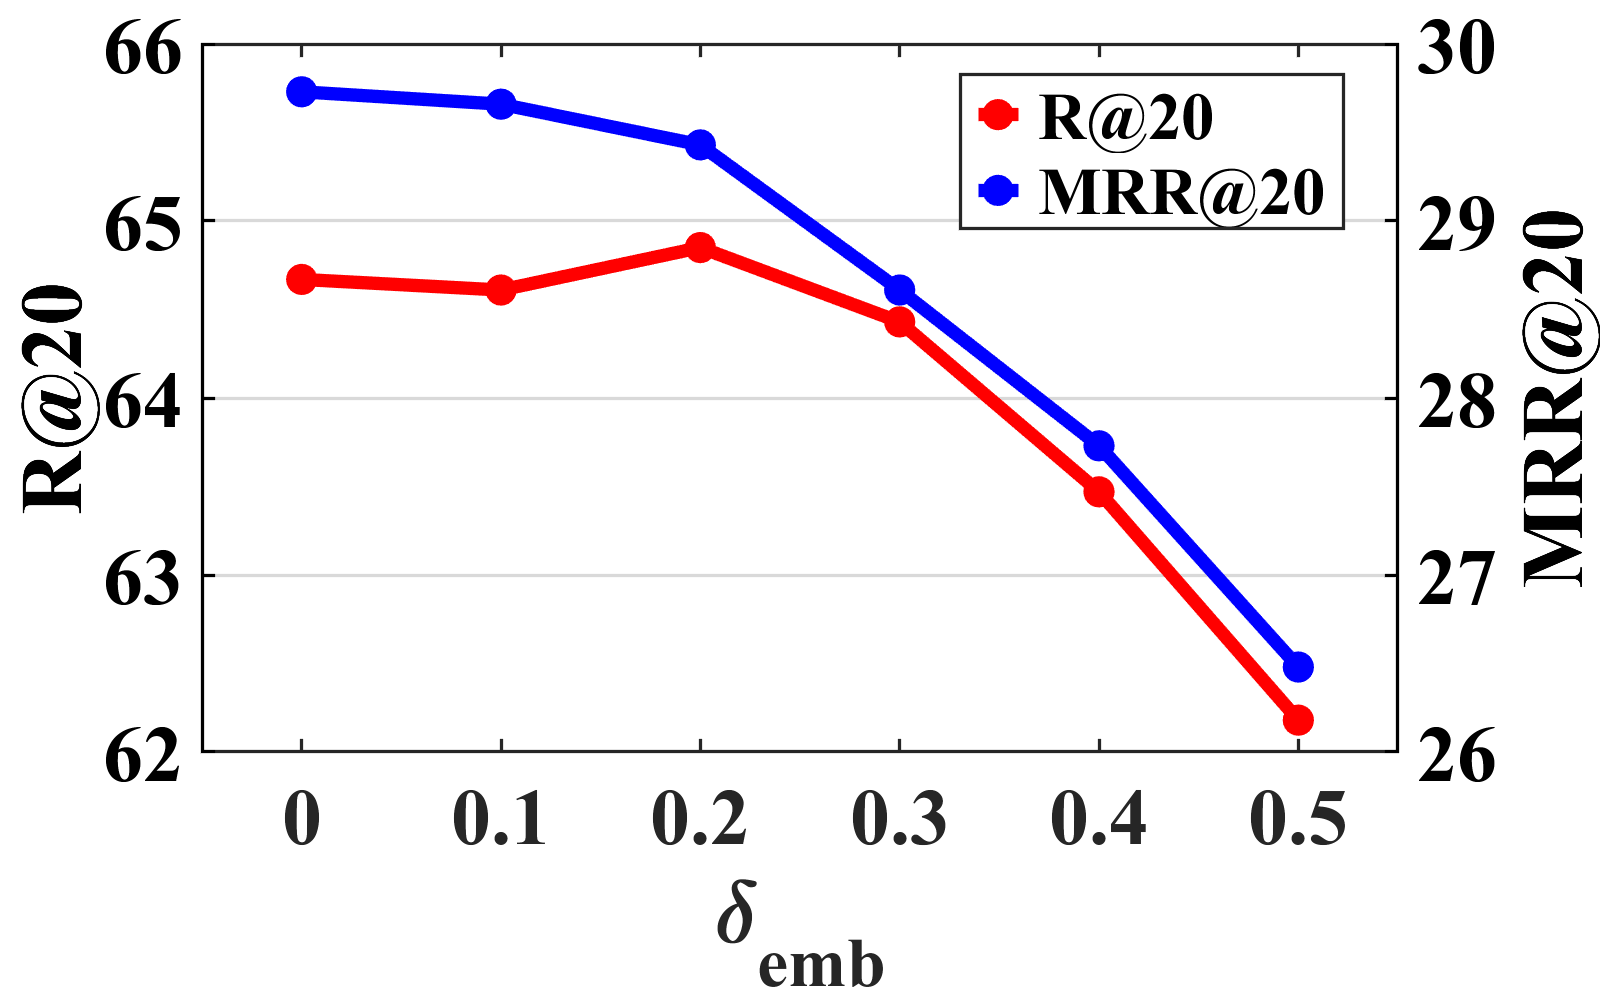}  &
\includegraphics[width=0.3\textwidth]{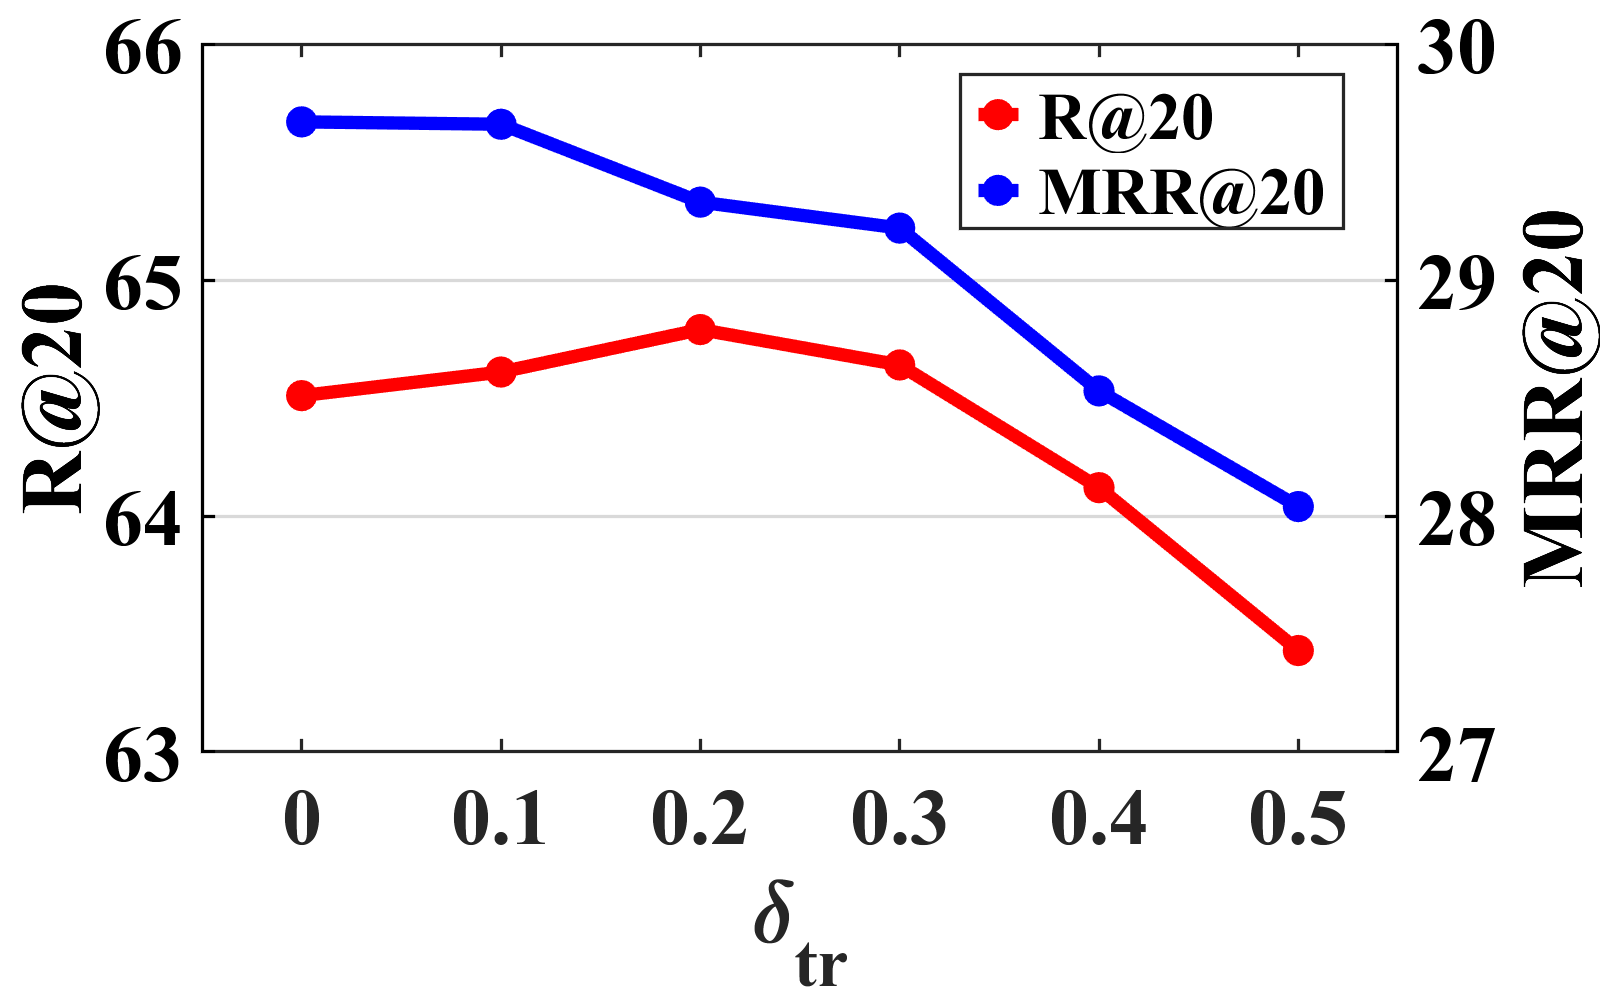} \\
\end{tabular} \\
(c) Yoochoose \\

\caption{Accuracy of EDISON over varying the hyperparameters: temperature $\tau$, embedding dropout ratio $\delta_{emb}$, and transformer layer dropout ratio $\delta_{tr}$.}
\label{fig:exp_hyperparameter}
\end{figure*}

% \includegraphics[width=1.0\linewidth]{Figures/empty.png}
% \caption{Parameter tuning of EDISON.}\label{fig:hyperparameter}
% \vskip -0.1in
% \end{figure}

Figure~\ref{fig:exp_hyperparameter} shows the effect of three hyperparameters of EDISON: temperature $\tau$ and dropout ratio for session/item vectors $\delta$. Temperature $\tau$ is more influential than the dropout ratio. When $\tau$ $\ge$ 0.5, EDISON shows a severe performance drop; it needs to be small enough for better convergence. EDISON shows the best performance when $\tau$ = 0.7 for both Retailrocket and Diginetica. When the dropout ratio $\delta$ is higher than 0.1, the higher the value, the worse the performance; it hinders model training. Setting the dropout ratio to 0.1 shows slightly better performance for the two datasets of Retailrocket and Diginetica. For the other datasets, the optimal value is low as 0 or 0.1.

\subsection{Analysis using an Optimal Extractor}\label{sec:exp_oracle}
% \begin{figure}[t]
% \centering
% \begin{tabular}{cc}
% \includegraphics[width=0.215\textwidth]{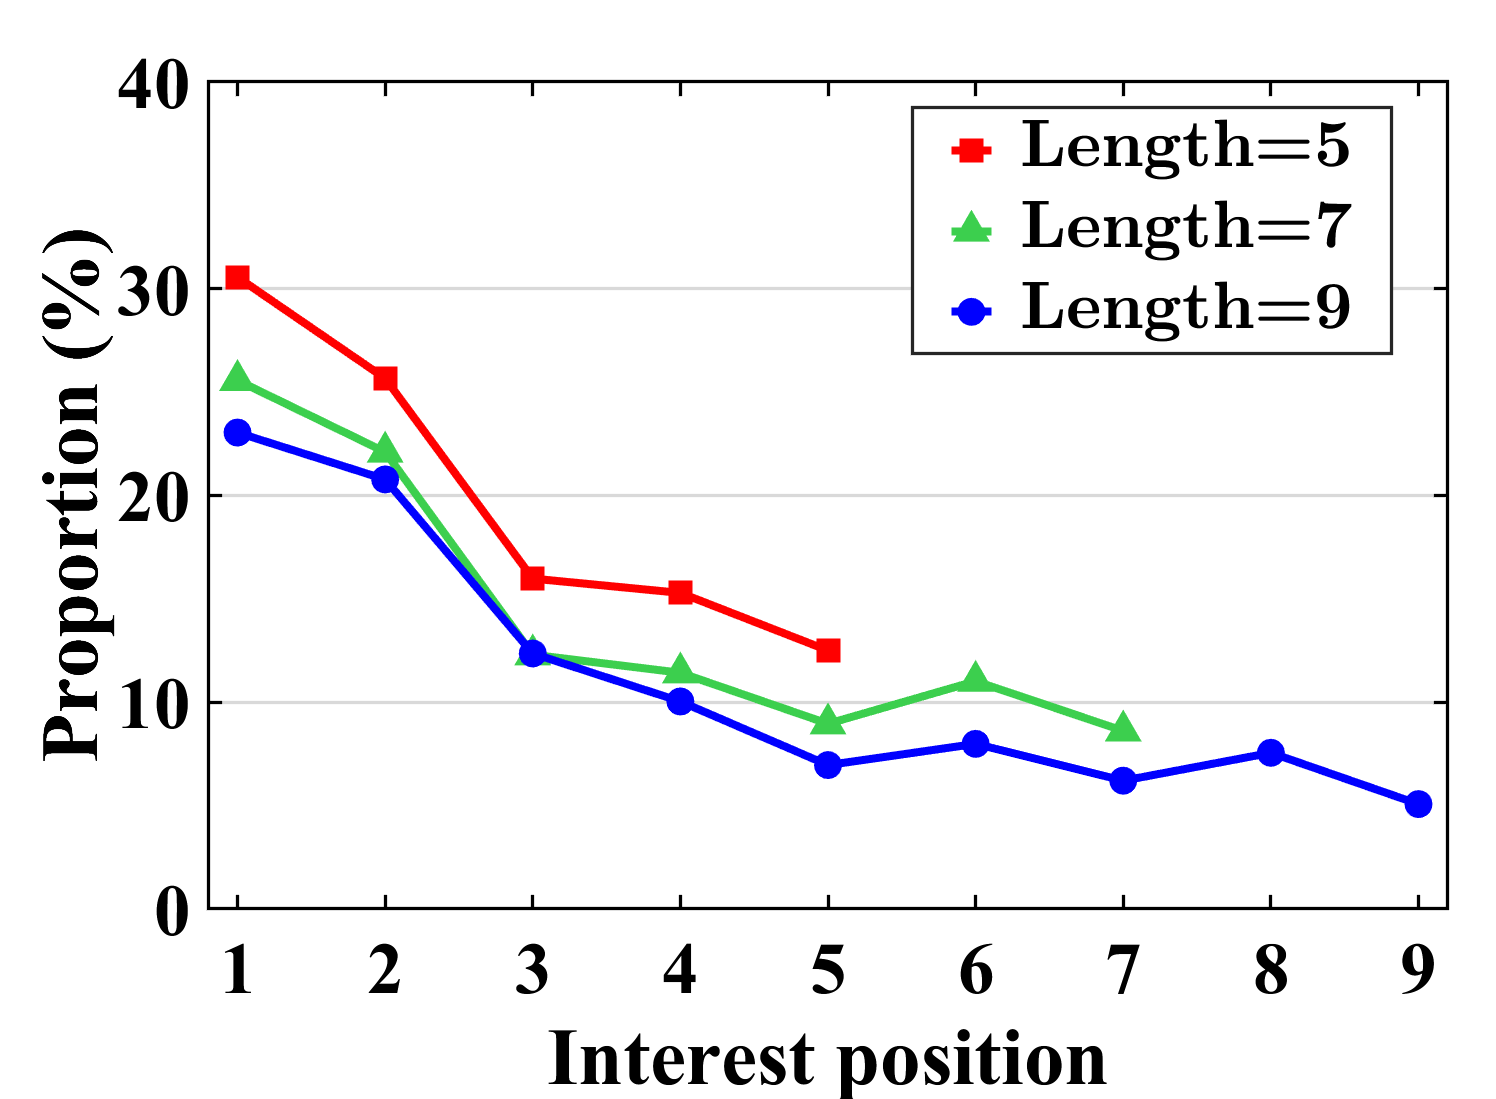} &
% \includegraphics[width=0.215\textwidth]{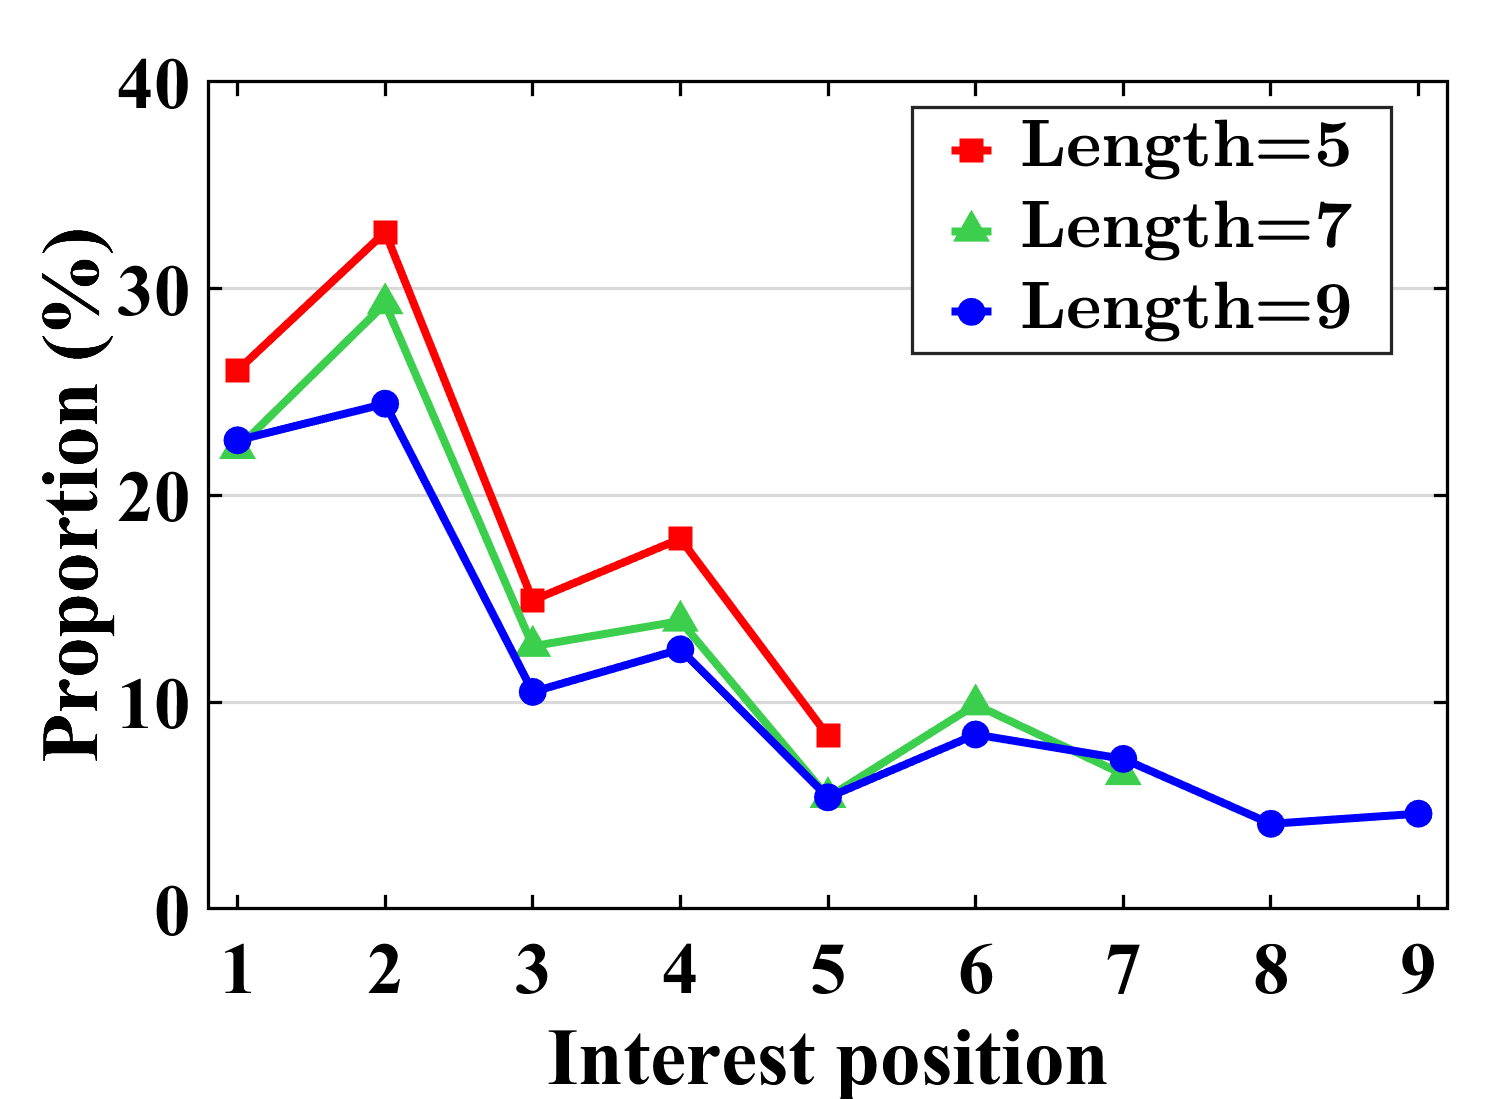}  \\
% % \includegraphics[width=0.28\textwidth]{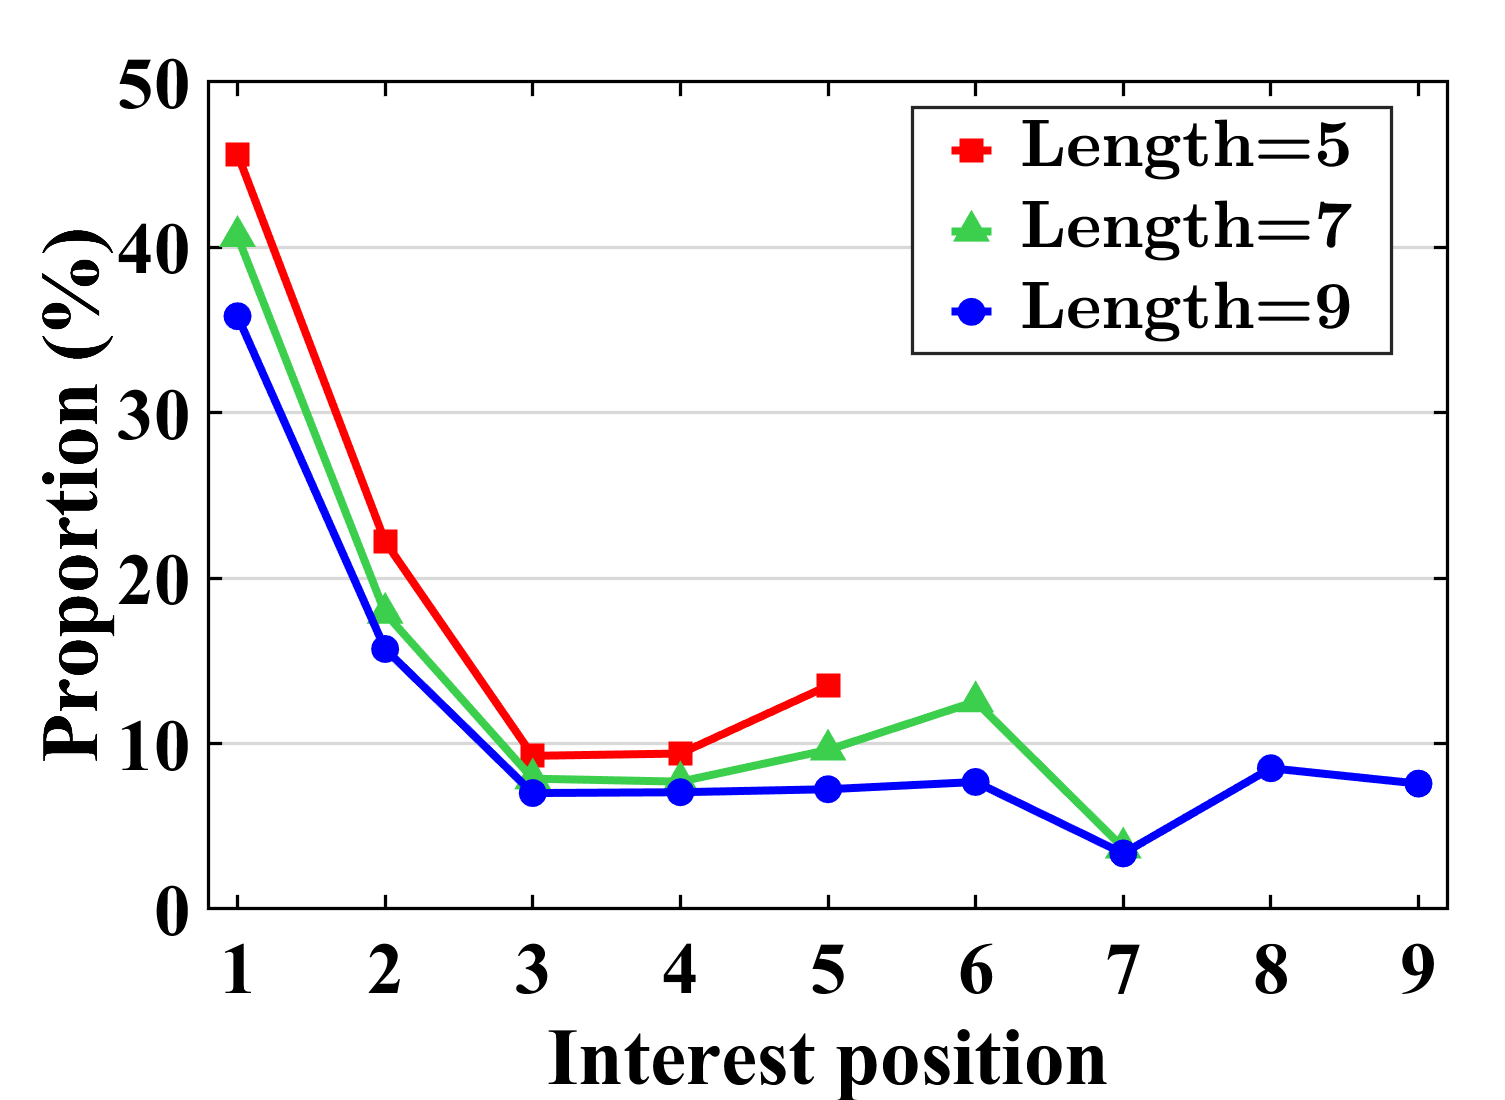} \\
% (a) Diginetica & (b) Retailrocket \\
% % \includegraphics[width=0.28\textwidth]{Figures/Tmall_oracle.png} &
% % \includegraphics[width=0.28\textwidth]{Figures/Dressipi_oracle.png}  & 
% % \includegraphics[width=0.28\textwidth]{Figures/LastFM_oracle.png} \\
% % (d) Tmall & (e) Dressipi & (f) LastFM\\

% \end{tabular}
% \caption{Distribution of user interests for long sessions using the optimal session extractor. The interest position indicates how far the user interest is from the last item (the last item is position 1).}\label{fig:exp_oracle_analysis}
% \end{figure}

\begin{figure*}[t]
\centering
\begin{tabular}{ccc}
\includegraphics[width=0.26\textwidth]{Figures/DIGI_oracle_v3.png} &
\includegraphics[width=0.26\textwidth]{Figures/RR_oracle_v3.png}  & 
\includegraphics[width=0.26\textwidth]{Figures/YC_oracle_v3.png} \\
(a) Diginetica & (b) Retailrocket & (c) Yoochoose \\
\includegraphics[width=0.26\textwidth]{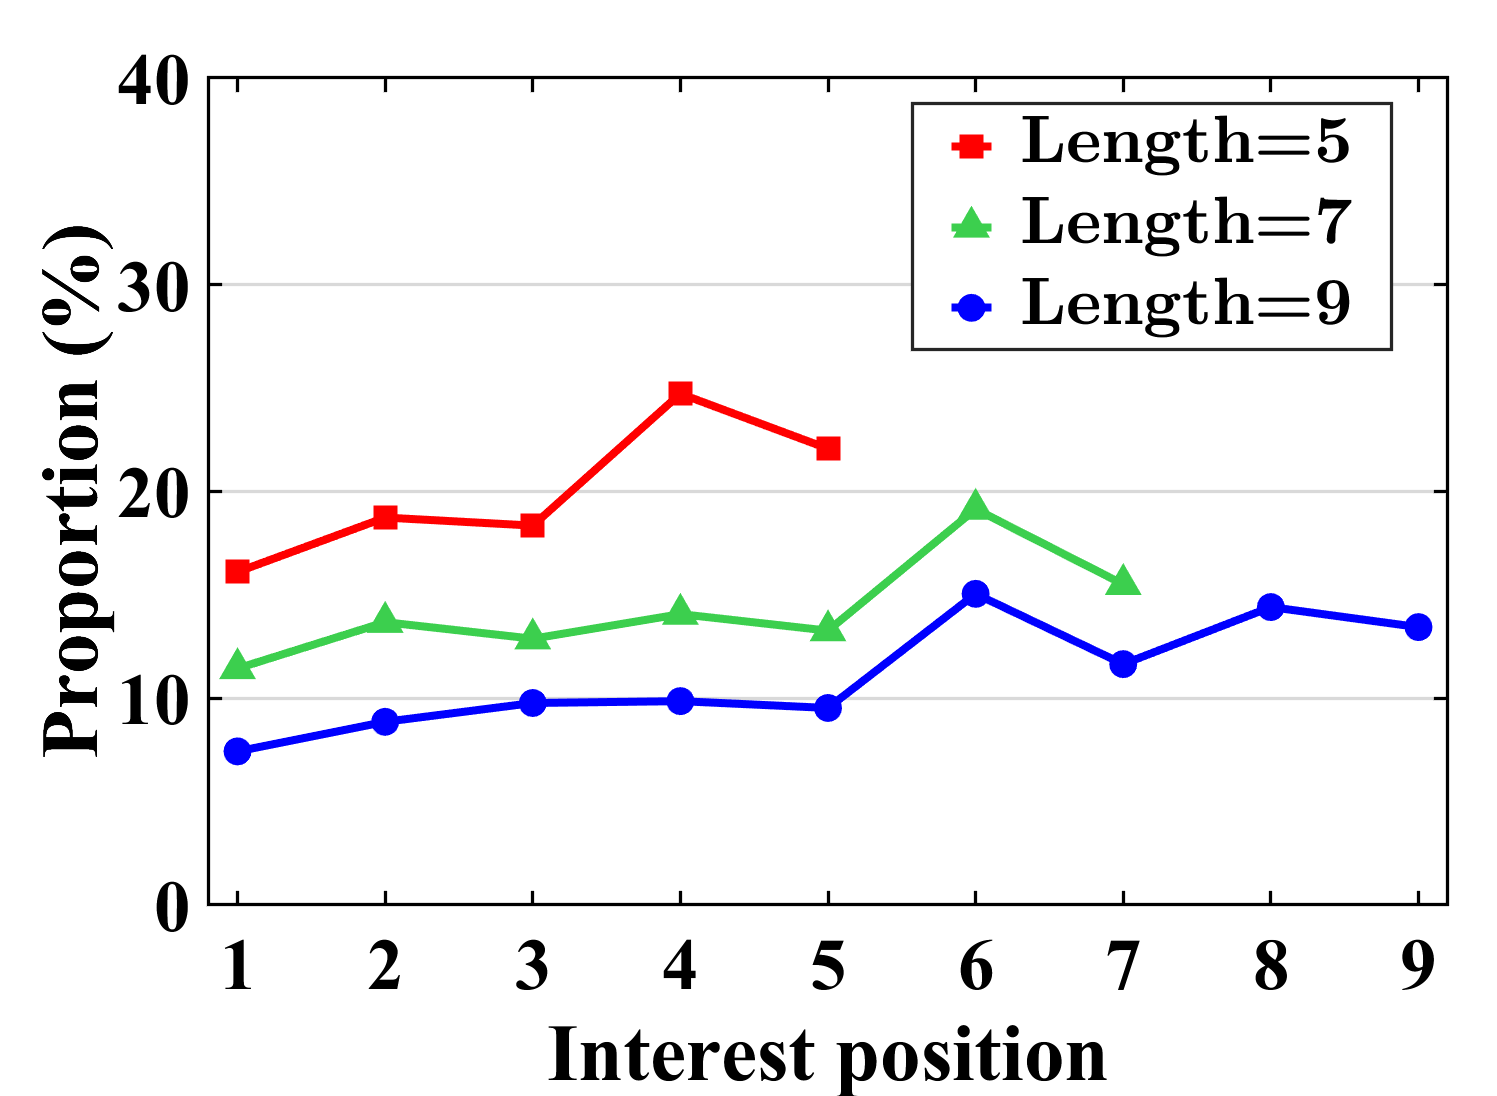} &
\includegraphics[width=0.26\textwidth]{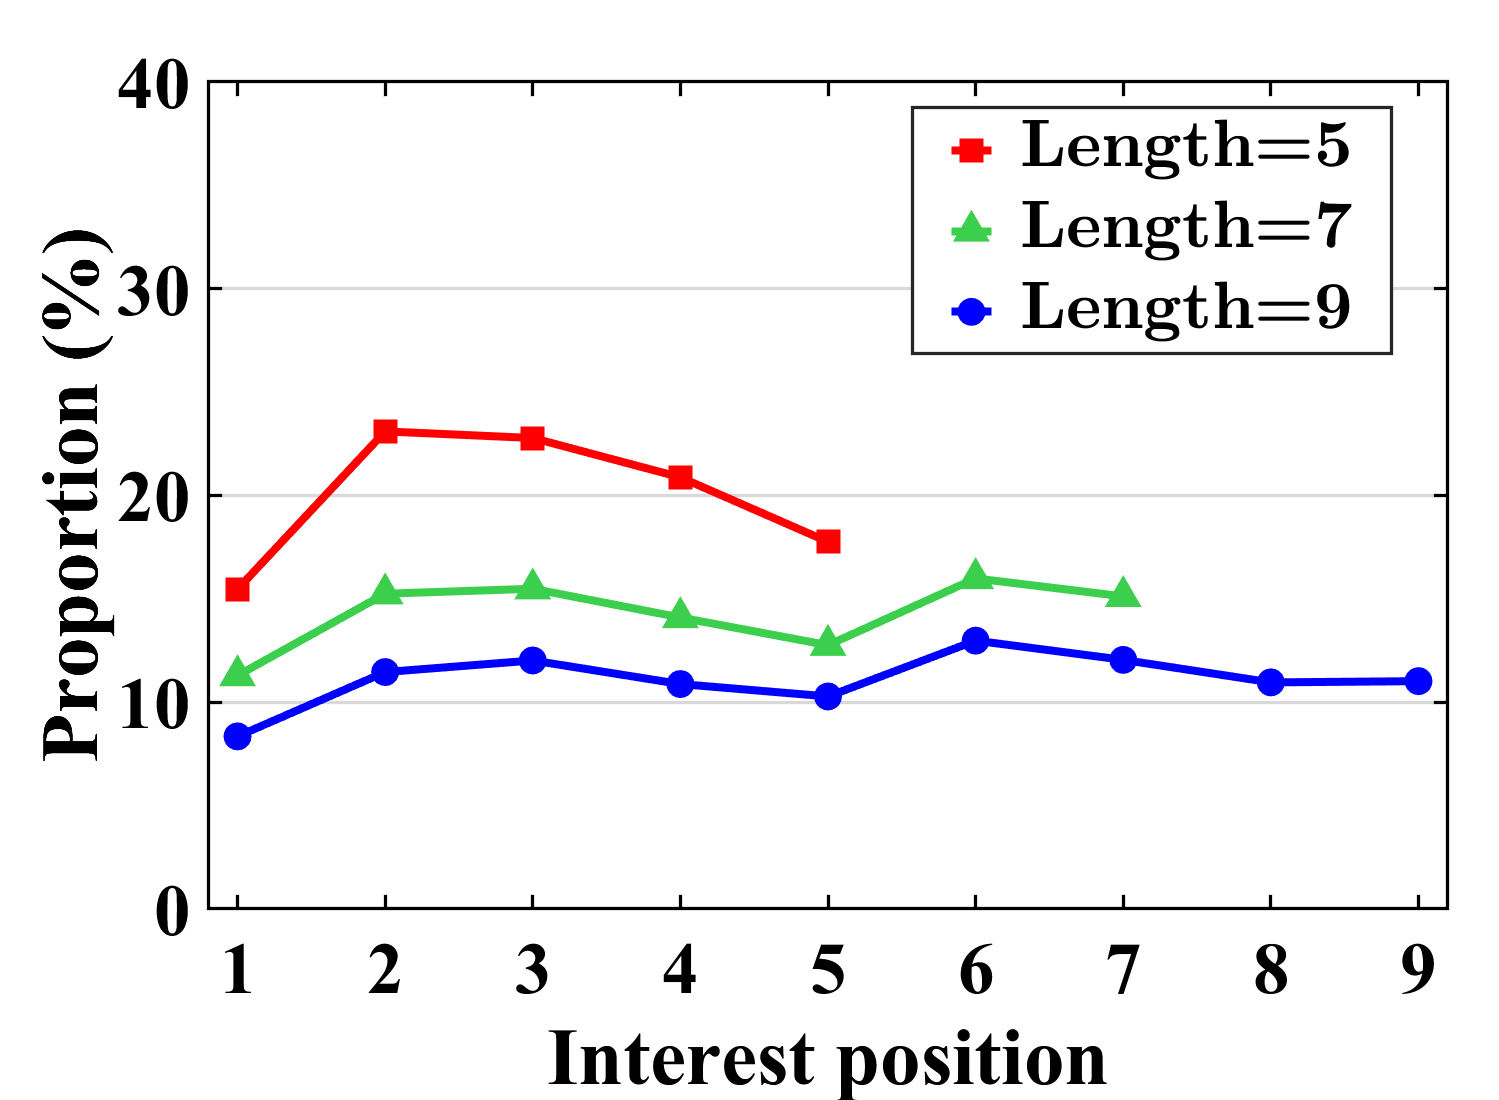}  & 
\includegraphics[width=0.26\textwidth]{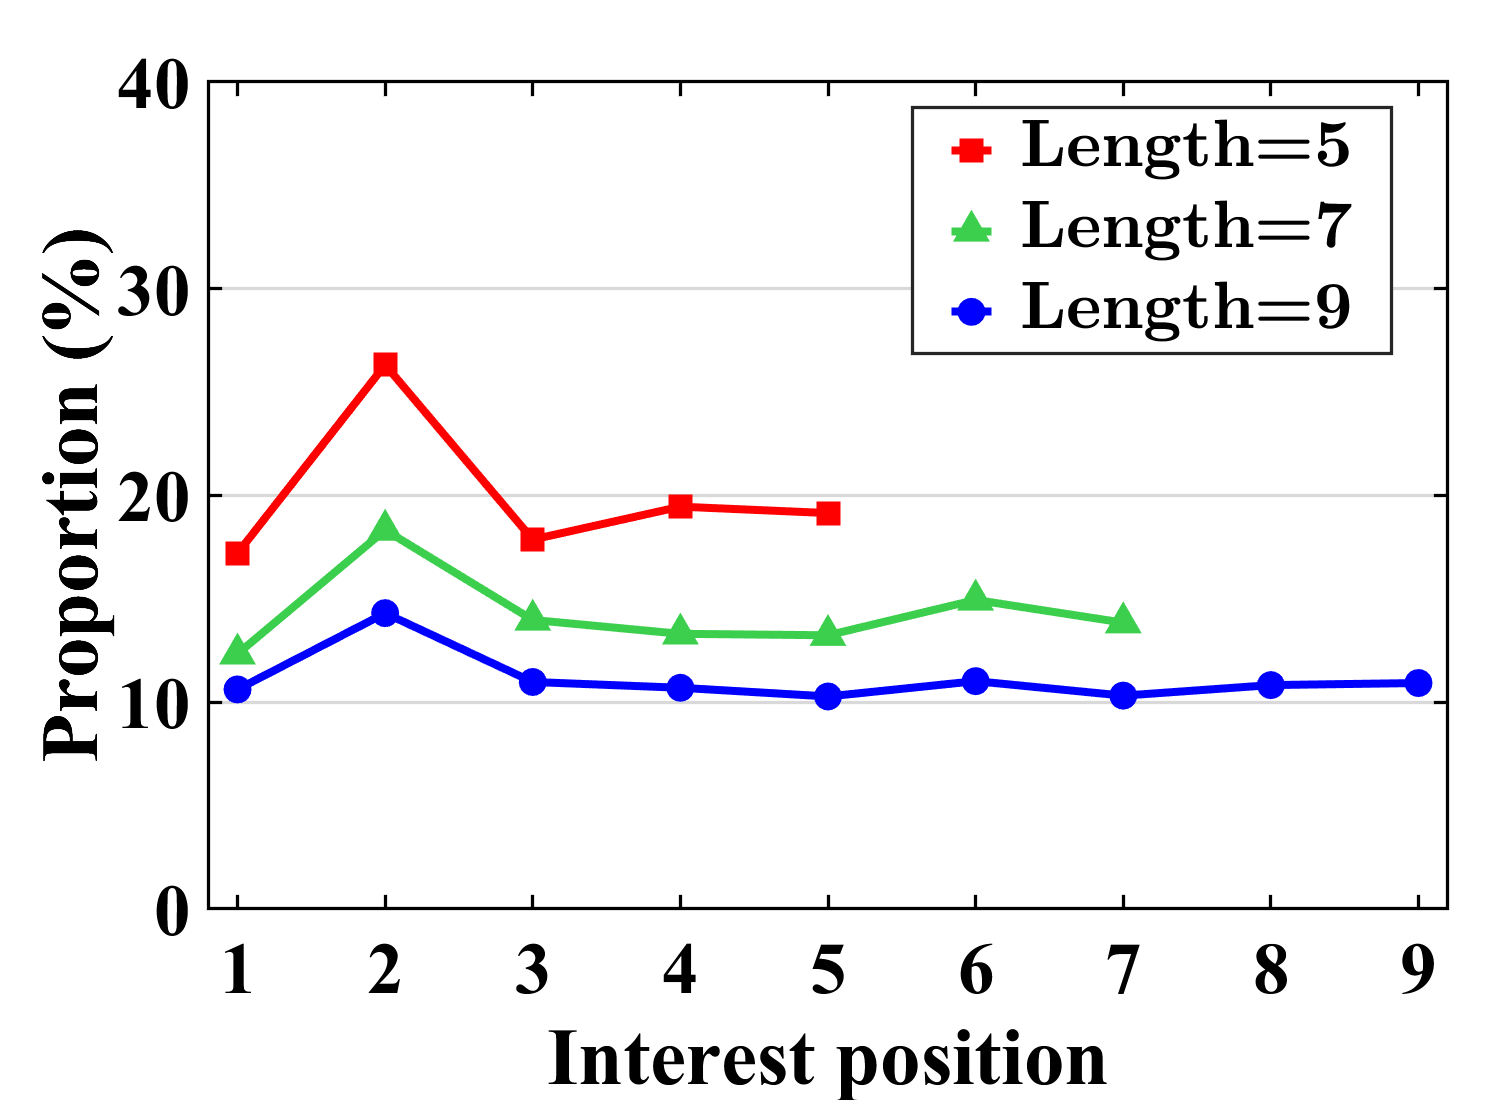} \\
(d) Tmall & (e) Dressipi & (f) LastFM \\

\end{tabular}
\caption{Distribution of user interests for long sessions using the optimal extractor. The interest position indicates how far the user interest is from the last item (the last item is position 1).}\label{fig:exp_oracle_analysis}
\end{figure*}

% \includegraphics[width=1.0\linewidth]{Figures/empty.png}
% \caption{Parameter tuning of EDISON.}\label{fig:hyperparameter}
% \vskip -0.1in
% \end{figure}

To analyze how diverse user interests are in a session, we assume that we know the target item in advance and devise an optimal extractor that points out the current interest among the various user interests. Given multiple session vectors representing user interests, the optimal extractor chooses the one most similar to the target item as the optimal session vector, supposing the current user interest corresponds to a target item. Let $\mathbf{v}_{\text{target}}$ be the embedding vector of the target item. Then we can extract the user interest as follows:
\begin{equation*}
\mathbf{h}_{\text{optimal}} =  \argmax_{\mathbf{c}_{i} \in \{\mathbf{c}_{1}, \dots, \mathbf{c}_{|s|}\}}cos(\mathbf{c}_{i}, \mathbf{v}_{\text{target}}). \\
\end{equation*}
\noindent
Figure~\ref{fig:exp_oracle_analysis} shows where user interest exists in a session with a specific length of five, seven, and nine. We can observe that the distribution is observed quite differently depending on the dataset. 

In Diginetica, the distribution of current user interest is relatively even across the sessions, making it difficult to determine which of multiple user interests is most important. For example, in approximately 43\% of sessions of length 5, the earlier three items (\eg, position 3, 4, and 5) reflect user interest. Meanwhile, Yoochoose shows a strong sequential dependency, where only about 32\% of sessions have user interest in the first three items, and about 45\% of sessions with length five have user interest in the last item, which is the closest in time. Among the three datasets, Retailrocket seems to have the least correlation between sequential order and user interest; the second last item most likely indicates user interest. These observations highlight the need to consider various user interests over the entire session by using multiple session representations.

Based on these observations, we stress that it is necessary to consider diverse user interests across the entire session. And, one of the best ways is using multiple session representations, as in EDISON. It consistently achieves the best performance regardless of session lengths since it selectively chooses an item as user interest irrespective of item positions. Meanwhile, existing SBR models mostly deal with the last item as user interest.

In the other three datasets, \eg, Tmall, Dressipi, and LastFM, user interest is observed throughout the session. For example, given a session of length 5 in these three datasets, the probability that a user interest exists in each location is more than 15\%. On the other hand, the datasets of Figure~\ref{fig:exp_oracle_analysis} show relatively strong sequential dependency, \eg, in Retailrocket, only 8\% of the cases in which the first item reflects the user's interest.

\begin{table}[] \small
\begin{tabular}{c|c|c}
\toprule
Model & \begin{tabular}[c]{@{}c@{}}Multiple\\ session vectors\end{tabular} & Aggregator \\ \midrule
\begin{tabular}[c]{@{}c@{}}
GRU4Rec, NARM, \\ 
SASRec, SR-GNN, \\ 
NISER+, SGNN-HN,\\ 
LESSR, CL4SRec, \\ 
CORE, Atten-mixer
\end{tabular} 
& \xmark & \xmark \\
\midrule
ComiRec, Re4 & fixed & max pooling \\ 
\midrule
EDISON (Ours) & adaptive & \begin{tabular}[c]{@{}c@{}} max-pooling + \\ average-pooling \end{tabular} \\ \bottomrule
\end{tabular}
\caption{Comparison of various session-based recommendation models and our proposed model, focusing on the main differences.}\label{tab:framework}
\end{table}

\iffalse

\begin{table}[] \small
\begin{tabular}{c|c|c}
\toprule
Model & \begin{tabular}[c]{@{}c@{}}Multiple\\ session vectors\end{tabular} & Aggregator \\ \midrule
\begin{tabular}[c]{@{}c@{}}
GRU4Rec~\cite{HidasiKBT15GRU4Rec, HidasiK18GRU4Rec+}, NARM~\cite{LiRCRLM17NARM}, \\ 
SASRec~\cite{KangM18SASRec}, SR-GNN~\cite{WuT0WXT19SRGNN}, \\ 
NISER+~\cite{GuptaGMVS19NISER}, SGNN-HN~\cite{PanCCCR20SGNNHN},\\ 
LESSR~\cite{ChenW20LESSR}, CL4SRec~\cite{XieSLWGZDC22CL4SRec}, \\ 
CORE~\cite{hou2022core}, Atten-mixer~\cite{ZhangGLXKZXWK23Atten-Mixer}
\end{tabular} 
& \xmark & \xmark \\
% \end{tabular} & \multirow{4}{*}{\xmark} & \multirow{4}{*}{\xmark} \\
% SR-GNN~\cite{WuT0WXT19SRGNN} & \cmark & \xmark & \xmark \\
% LESSR~\cite{ChenW20LESSR} & \cmark & \xmark & \xmark \\
% NISER+~\cite{GuptaGMVS19NISER} & \cmark & \xmark & \xmark \\
% SGNN-HN~\cite{PanCCCR20SGNNHN} & \cmark & \xmark & \xmark \\
% SASRec~\cite{KangM18SASRec} & \cmark & \xmark & \xmark \\
% CL4SRec~\cite{XieSLWGZDC22CL4SRec} & \cmark & \xmark & \xmark \\
% CORE~\cite{hou2022core} & \cmark & \xmark & \xmark \\
% A-mixer~\cite{ZhangGLXKZXWK23Atten-Mixer} & \cmark & \xmark & \xmark \\
\midrule
% ComiRec~\cite{ChenZZXX21ComiRec} & \cmark & Fixed & Max pool \\
ComiRec~\cite{ChenZZXX21ComiRec}, Re4~\cite{ZhangYYLFZC022Re4} & fixed & max pooling \\ 
\midrule
% EDISON(Ours) & + $\mathbf{v}_{\text{mean}}$ & Adaptive & Max+Avg pool \\ \bottomrule
% EDISON (Ours) & Adaptive & \begin{tabular}[c]{@{}c@{}} Max-pooling + \\ Average-pooling \end{tabular} \\ \bottomrule
EDISON (Ours) & \begin{tabular}[c]{@{}c@{}} adaptive by \\ session length \end{tabular} & \begin{tabular}[c]{@{}c@{}} max-pooling + \\ average-pooling \end{tabular} \\ \bottomrule
\end{tabular}
\caption{Comparison of various session-based recommendation models and our proposed model, focusing on the main differences.}\label{tab:framework}
\end{table}

\fi
